# Supplementary material for: VEIGAR: View-consistent Explicit Inpainting and Geometry Alignment for 3D object Removal
Source: arXiv:2506.15821 source file (2025-06-13)
Supplement: Supplementary file 1 [file implementation.tex]

In our implementation, we employ DUST3R \cite{Wang_2024_CVPR} to estimate depth maps from stereo images, and DepthAnythingV2 \cite{yang2024depth} as a monocular depth estimator. The depth outputs from both methods are subsequently fused using a lightweight multi-layer perceptron (MLP) to generate a unified depth representation. For implicit intrinsic alignment, we define $\tilde{\mathbf{K}}$ as another lightweight MLP to ensure comprehensive projection, followed by optimization.

For the inpainting task, we utilize LaMa \cite{suvorov2022resolution} to complete the missing regions, which are then input into the 3D reconstruction pipeline. During 3D supervision, we apply a scale-invariant depth loss with a weighting factor $ \lambda = 0.5$ to balance the loss terms. Additionally, for the Gaussian splatting, we set $ \lambda_{\text{color}} = 0.8$ and $ \lambda_{\text{ssim}} = 0.2$ to further refine the reconstruction.

\paragraph{Evaluation settings} We compute LoFTR scores over 100 randomly sampled pairs of test images per scene. To account for domain-specific performance, we apply LoFTR with indoor pre-trained weights for the "book," "trash," and "9" scenes, while using outdoor weights for the remaining ones. A matching confidence threshold of 0.95 is applied to filter LoFTR correspondences during evaluation.
