# Supplementary material for: VEIGAR: View-consistent Explicit Inpainting and Geometry Alignment for 3D object Removal
Source: arXiv:2506.15821 source file (2025-06-13)
Supplement: Supplementary file 2 [file inpainter.tex]

As shown in Fig.\ref{fig:inpainter}, MVInpainter delivers visually coherent inpainting results that align well with human perception. However, in downstream reconstruction tasks such as 3D Gaussian Splatting (3DGS), which require strict pixel-level alignment across views, differences in inpainting quality can become more apparent. One contributing factor is the fixed output resolution of 512×512 used by MVInpainter, which may lead to the loss of high-frequency details present in the original images. Similarly, In-and-Out incorporates latent alignment mechanisms to maintain cross-view consistency, yet performance can still be impacted when anchor views diverge significantly from their original appearance, as illustrated in the example scenes. In our approach, we experiment with using SDXL for inpainting the masked regions identified in the first stage. While effective in many cases, SDXL can occasionally misinterpret binary masks as semantic cues, resulting in residual artifacts that follow the shape of the masks. By contrast, when using LaMa for inpainting, our method produces high-resolution, clean, and semantically consistent outputs that better meet the pixel-level alignment requirements of 3DGS, contributing to improved reconstruction fidelity.

\begin{figure}
\centering
\setlength{\tabcolsep}{4pt}

\begin{tabular}{c|c|c|c}
 & \textbf{Scene Book} & \textbf{Scene Trash} & \textbf{Scene 1} \\
\hline
\parbox[c][3.0cm][c]{0.3cm}{\centering\rotatebox{90}{MV-Inpainter}} & 
\begin{tabular}{c}
\includegraphics[width=0.27\linewidth]{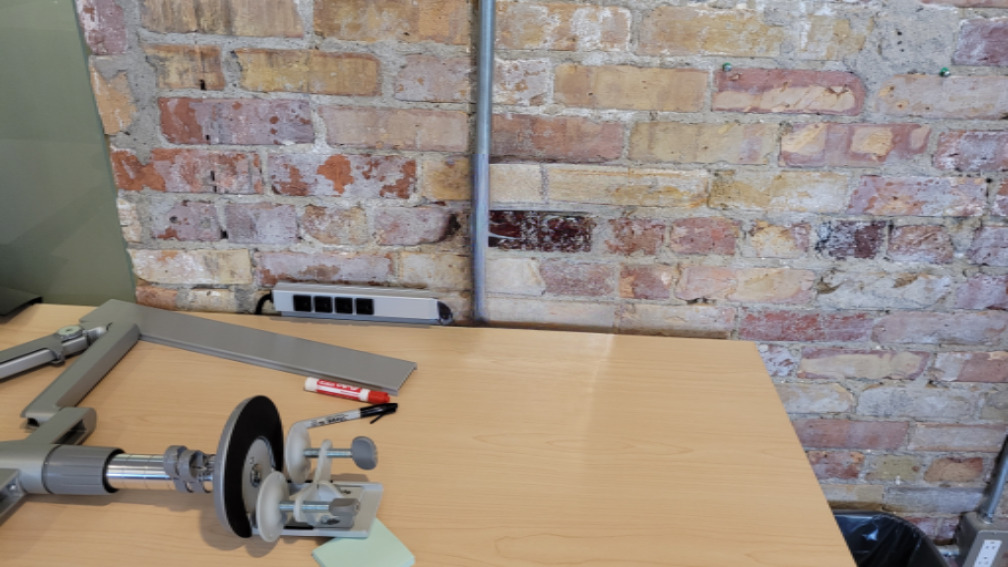} \\[-4pt]
\includegraphics[width=0.27\linewidth]{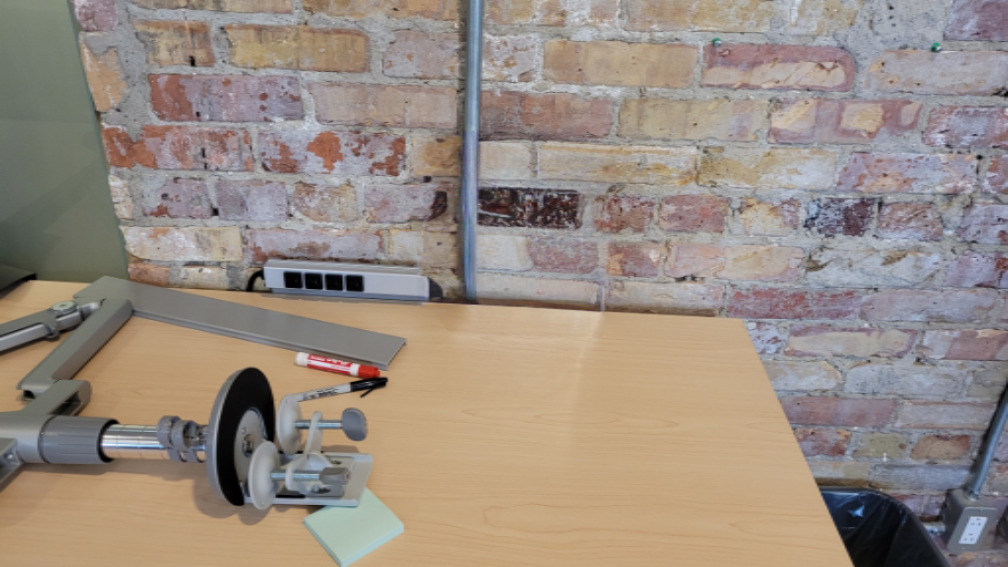}
\end{tabular} &
\begin{tabular}{c}
\includegraphics[width=0.27\linewidth]{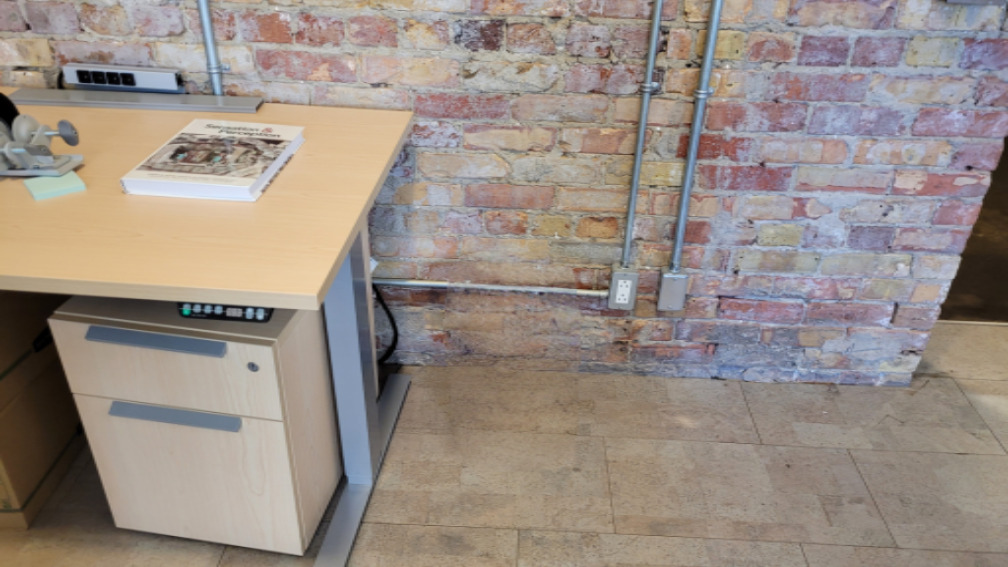} \\[-4pt]
\includegraphics[width=0.27\linewidth]{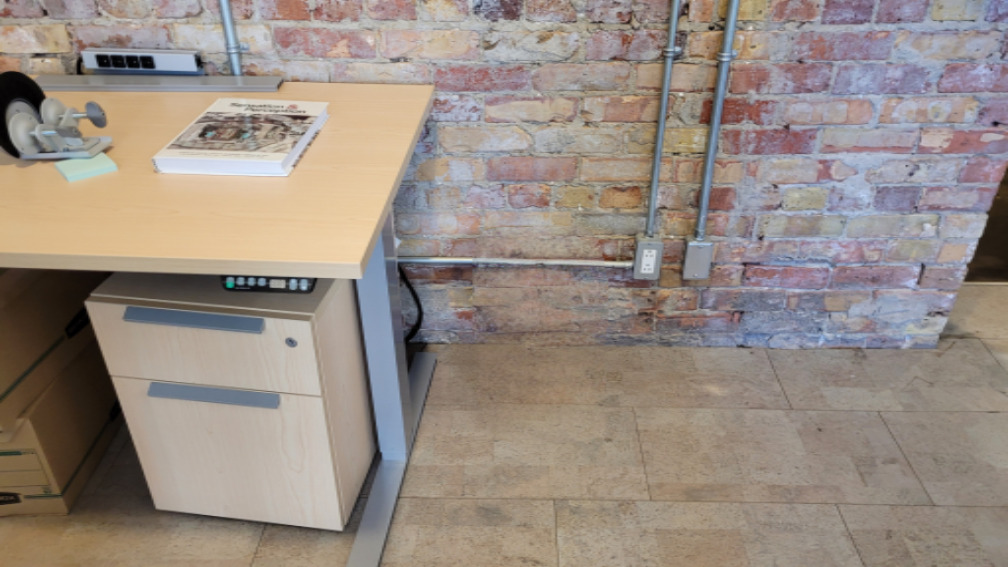}
\end{tabular} &
\begin{tabular}{c}
\includegraphics[width=0.27\linewidth]{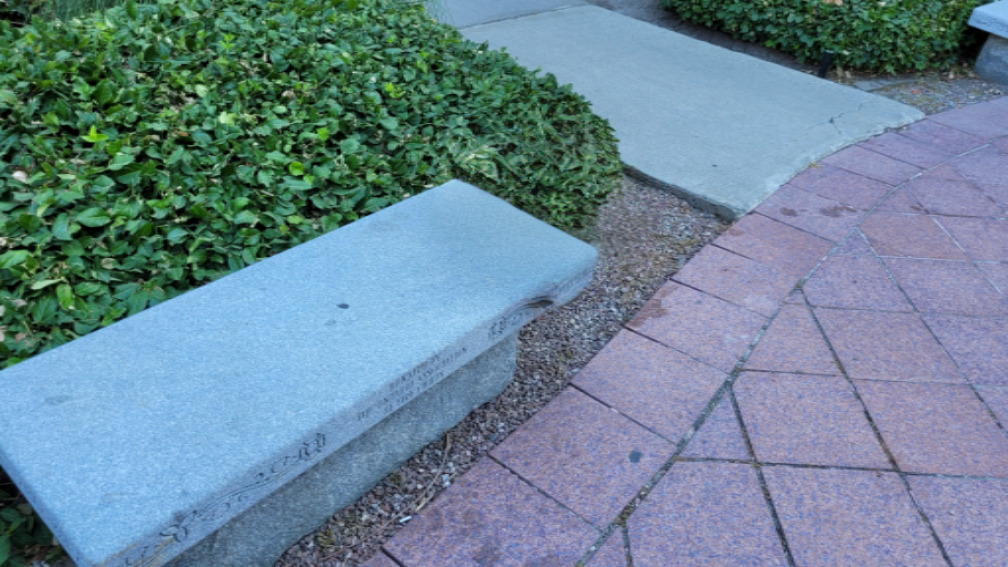} \\[-4pt]
\includegraphics[width=0.27\linewidth]{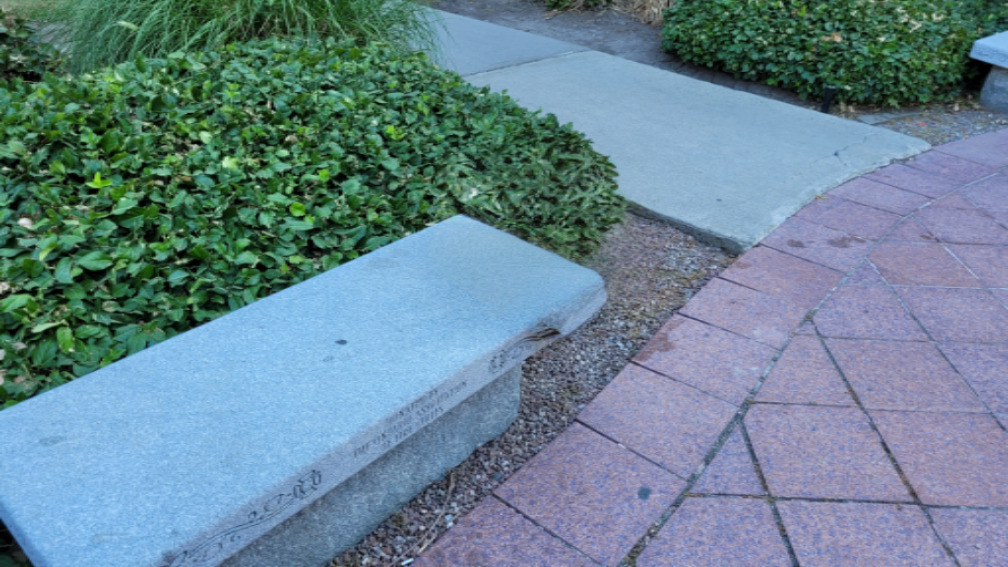}
\end{tabular} \\

\parbox[c][3.0cm][c]{0.3cm}{\centering\rotatebox{90}{In-and-Out}} & 
\begin{tabular}{c}
\includegraphics[width=0.27\linewidth]{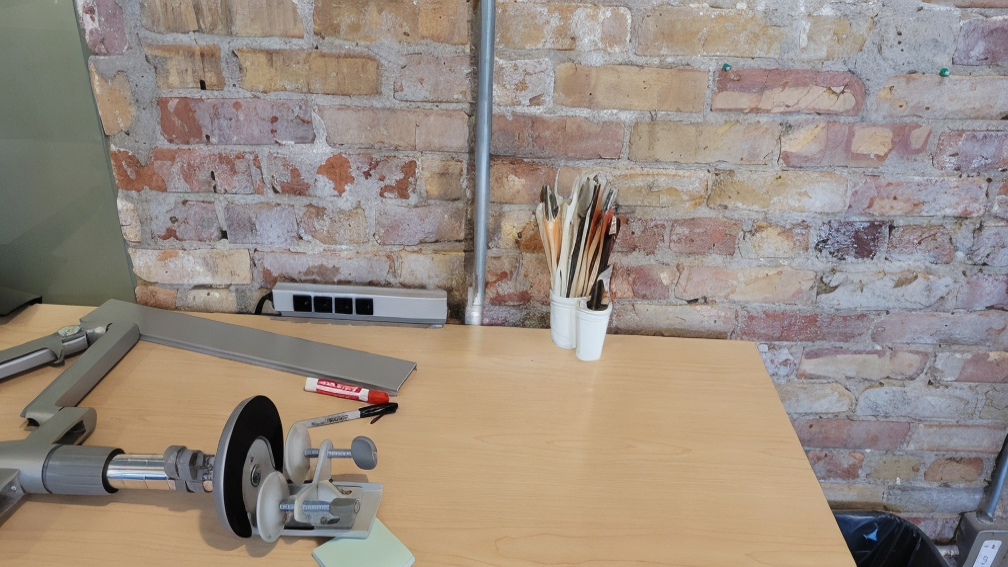} \\[-4pt]
\includegraphics[width=0.27\linewidth]{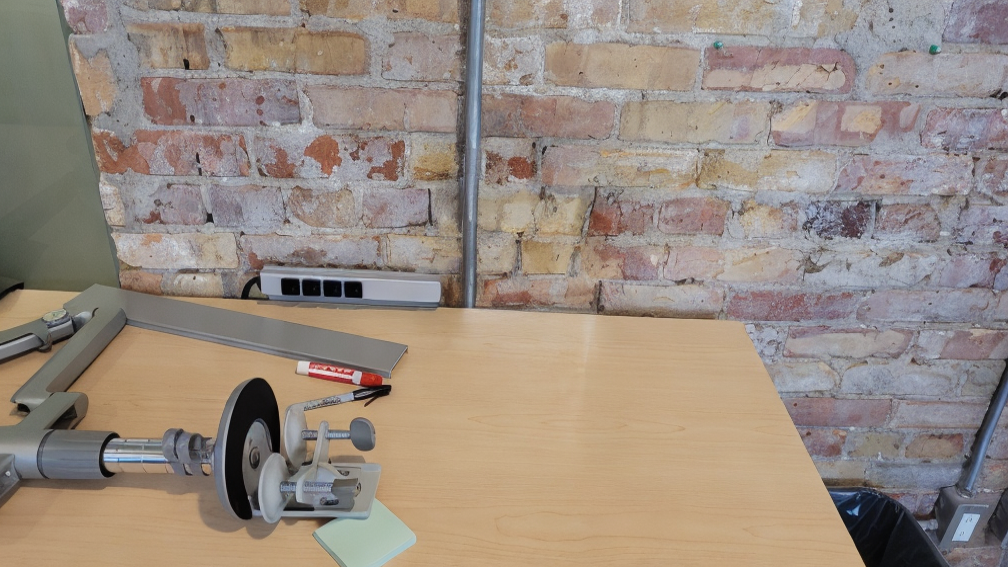}
\end{tabular} &
\begin{tabular}{c}
\includegraphics[width=0.27\linewidth]{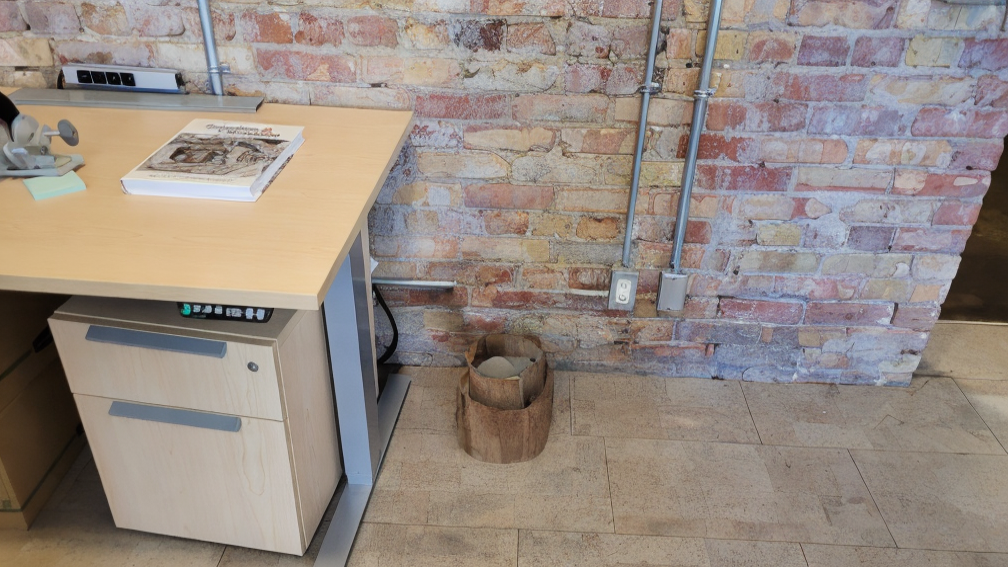} \\[-4pt]
\includegraphics[width=0.27\linewidth]{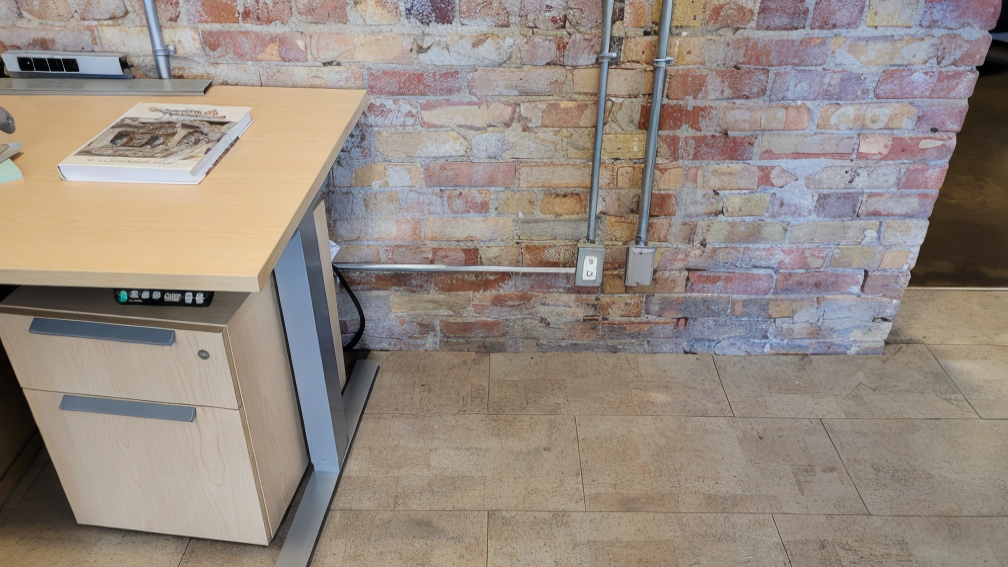}
\end{tabular} &
\begin{tabular}{c}
\includegraphics[width=0.27\linewidth]{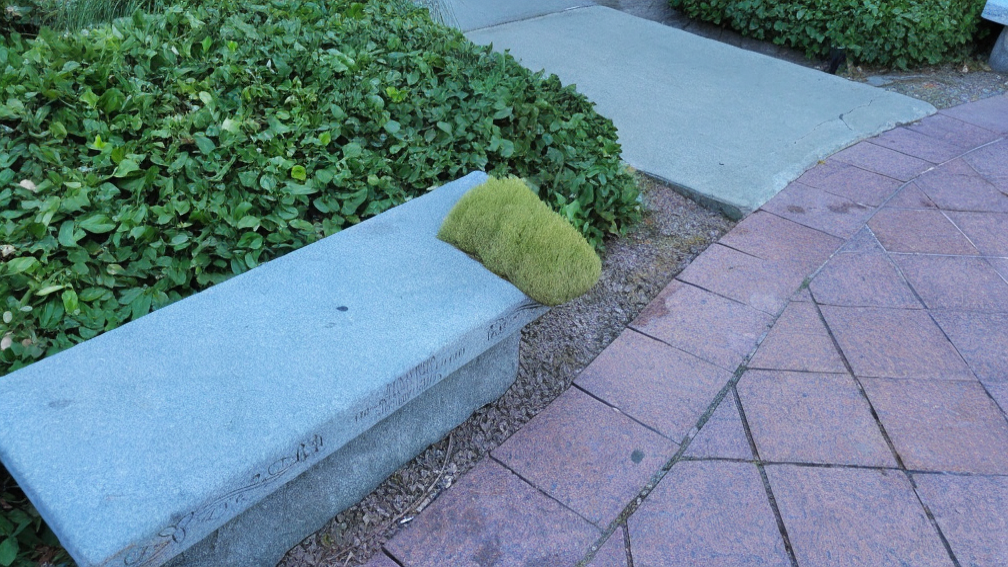} \\[-4pt]
\includegraphics[width=0.27\linewidth]{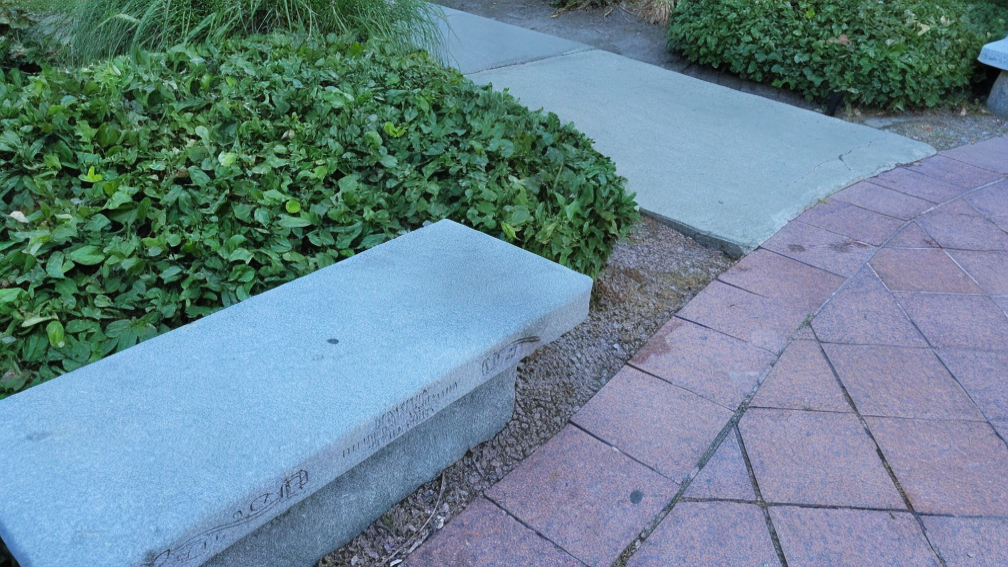}
\end{tabular} \\

\parbox[c][3.0cm][c]{0.3cm}{\centering\rotatebox{90}{Ours (SDXL)}} & 
\begin{tabular}{c}
\includegraphics[width=0.27\linewidth]{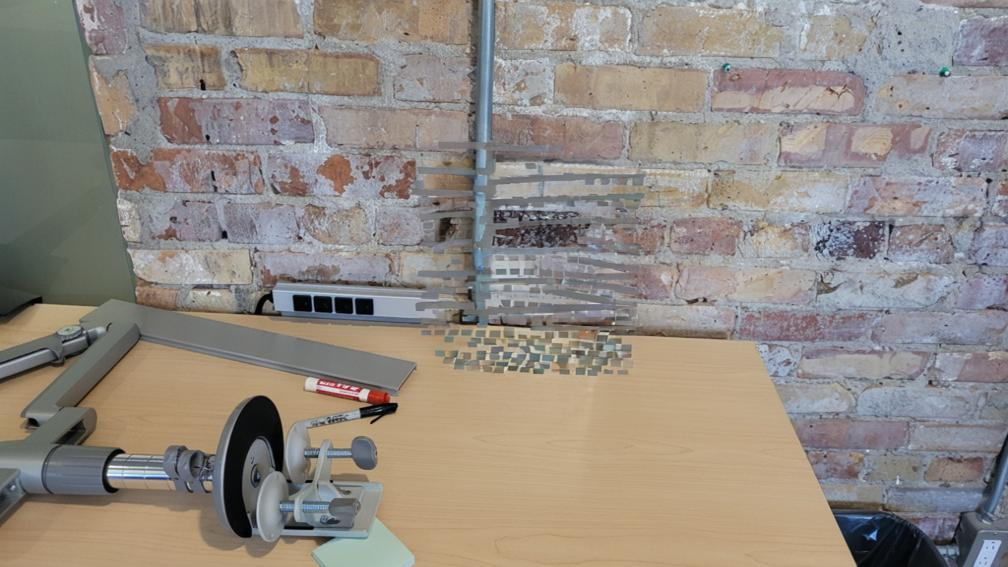} \\[-4pt]
\includegraphics[width=0.27\linewidth]{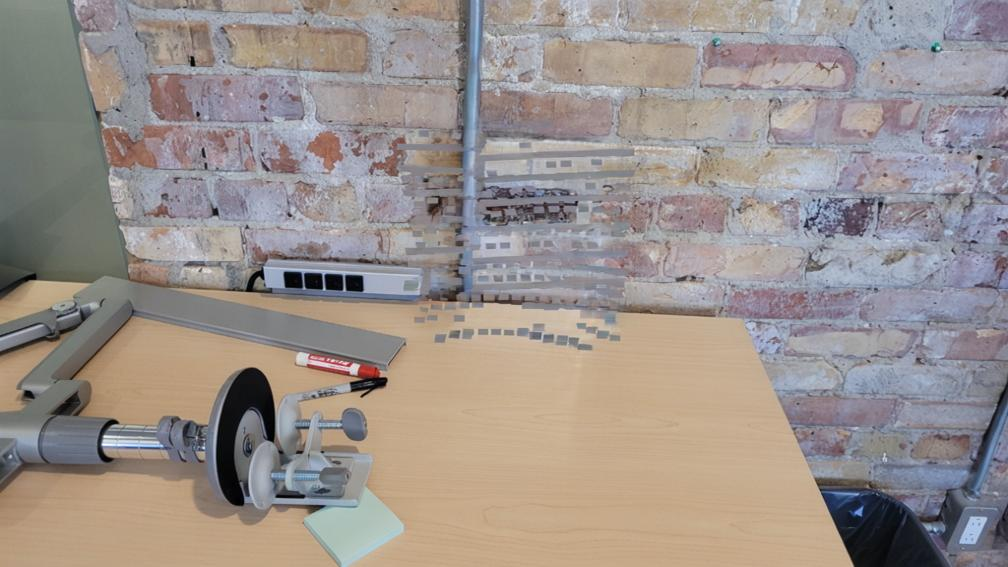}
\end{tabular} &
\begin{tabular}{c}
\includegraphics[width=0.27\linewidth]{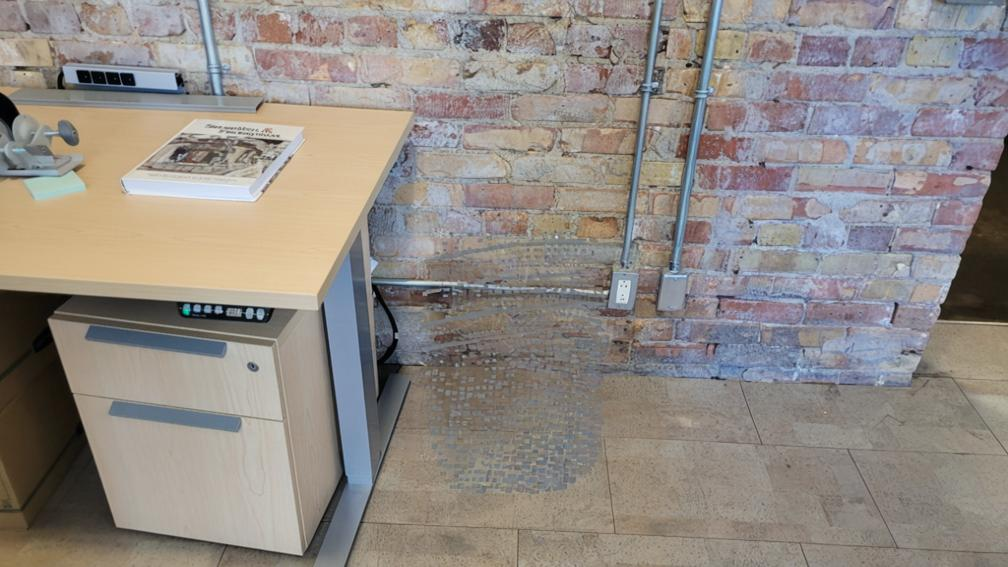} \\[-4pt]
\includegraphics[width=0.27\linewidth]{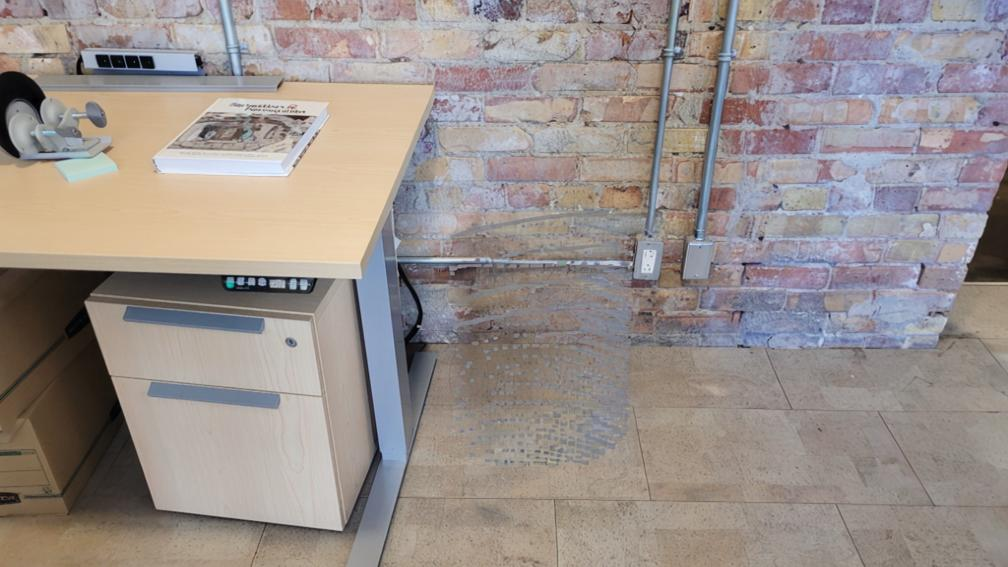}
\end{tabular} &
\begin{tabular}{c}
\includegraphics[width=0.27\linewidth]{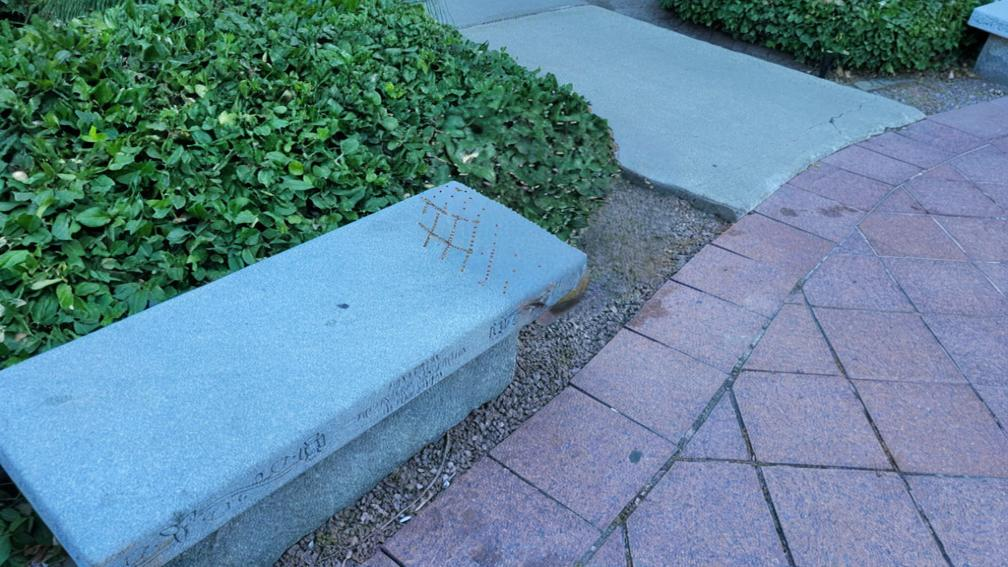} \\[-4pt]
\includegraphics[width=0.27\linewidth]{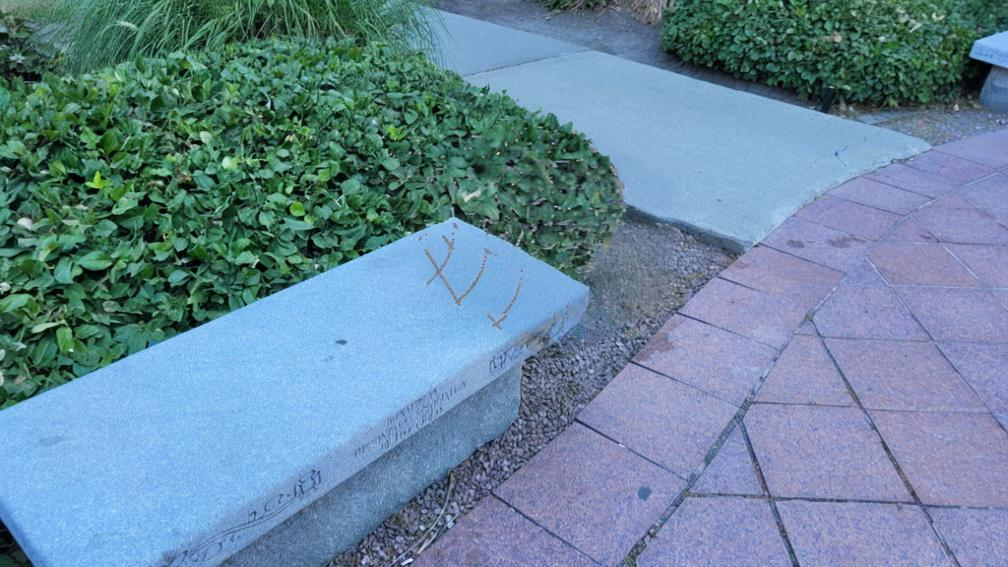}
\end{tabular} \\
\parbox[c][3.0cm][c]{0.3cm}{\centering\rotatebox{90}{Ours (LaMa)}} & 
\begin{tabular}{c}
\includegraphics[width=0.27\linewidth]{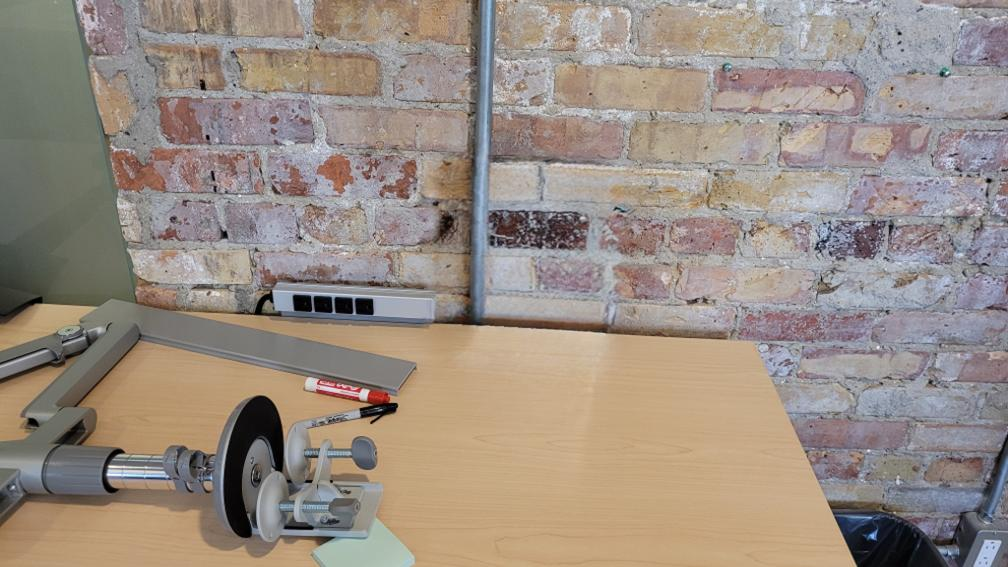} \\[-4pt]
\includegraphics[width=0.27\linewidth]{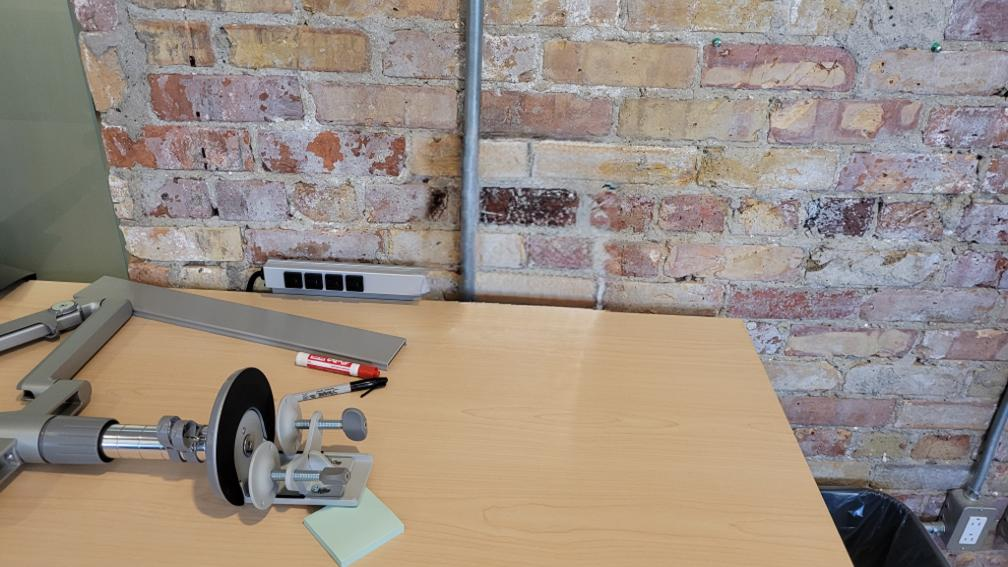}
\end{tabular} &
\begin{tabular}{c}
\includegraphics[width=0.27\linewidth]{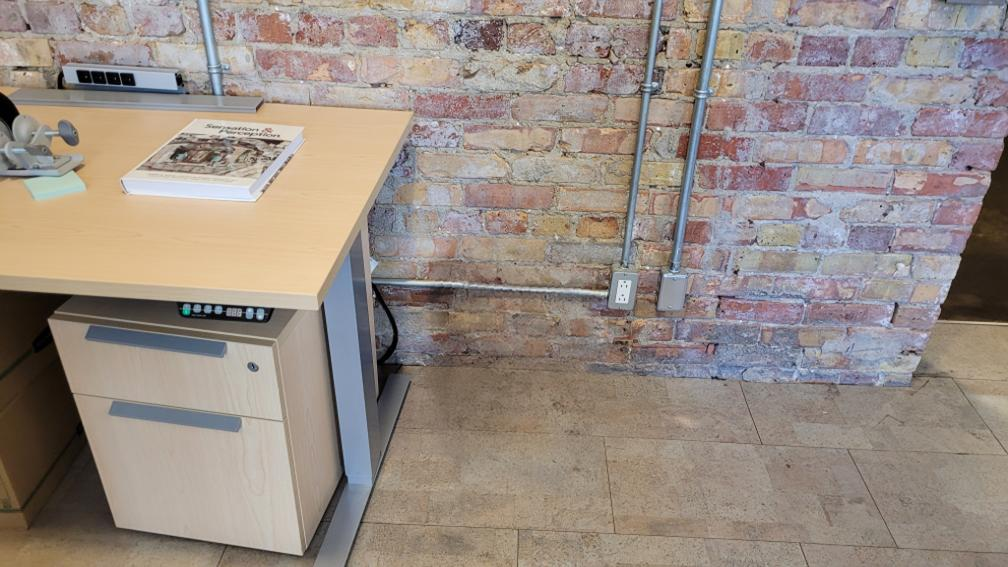} \\[-4pt]
\includegraphics[width=0.27\linewidth]{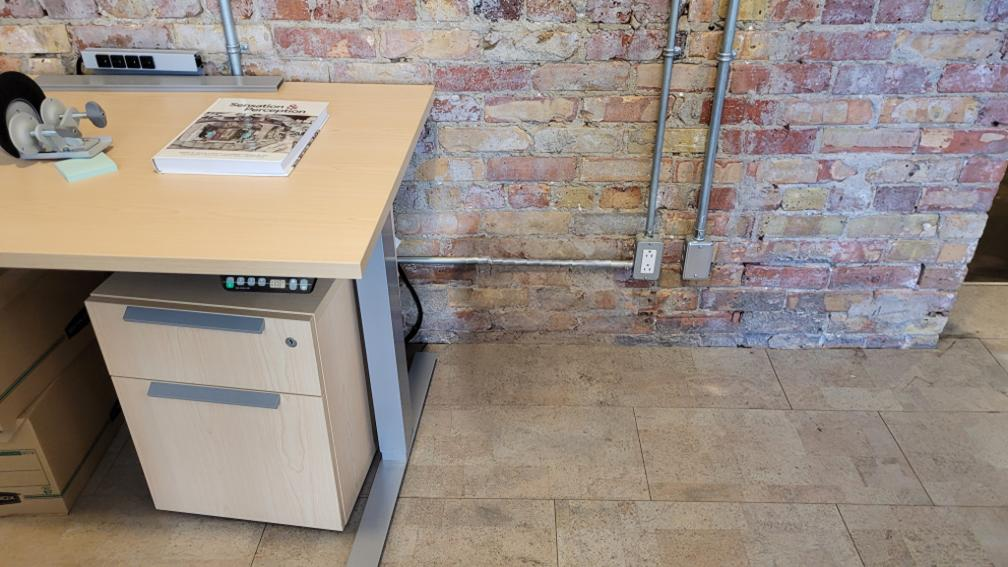}
\end{tabular} &
\begin{tabular}{c}
\includegraphics[width=0.27\linewidth]{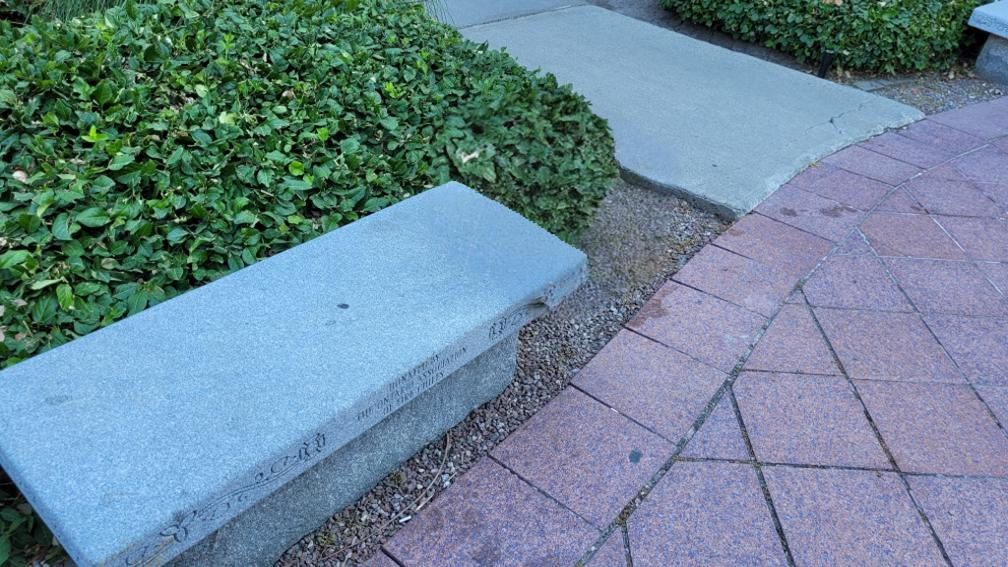} \\[-4pt]
\includegraphics[width=0.27\linewidth]{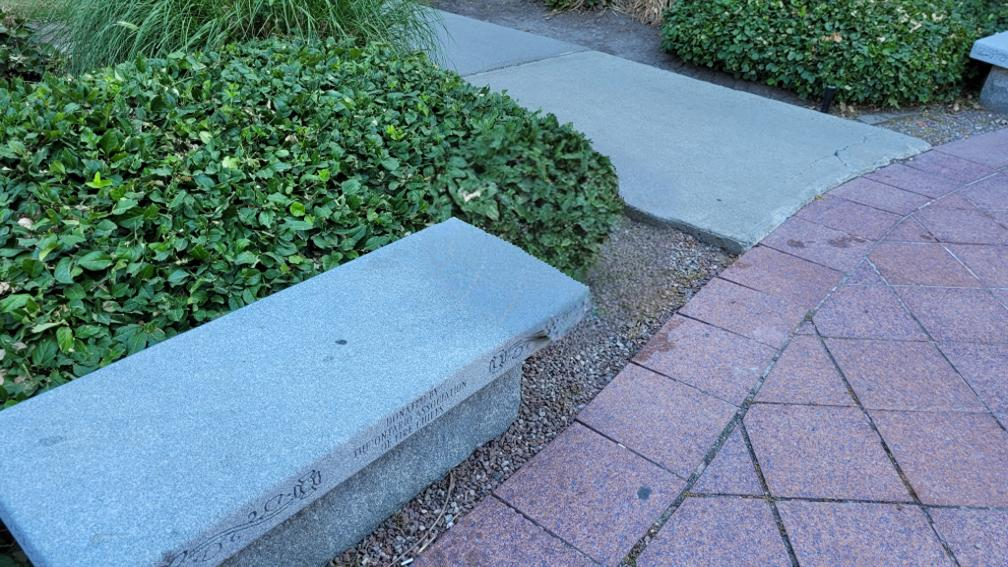}
\end{tabular} \\
\end{tabular}

\caption[Comparison of vertically stacked inpainting results]{Qualitative comparison of inpainting results across three scenes. Each cell shows two vertically stacked views for a given method and scene.}
\label{fig:inpainter}
\end{figure}
