# Supplementary material for: VEIGAR: View-consistent Explicit Inpainting and Geometry Alignment for 3D object Removal
Source: arXiv:2506.15821 source file (2025-06-13)
Supplement: Supplementary file 3 [file si.tex]

The \textit{Scale-Invariant Logarithmic Loss}, introduced in the context of monocular depth estimation, is defined as:
\begin{equation}
    L(\hat{d}, d) = \frac{1}{n} \sum_{p} \left( \ln \hat{d}_p - \ln d_p \right)^2 - \frac{1}{n^2} \left( \sum_{p} \left( \ln \hat{d}_p - \ln d_p \right) \right)^2,
\end{equation}
where \( \hat{d}_p \) and \( d_p \) denote the predicted and ground truth depth at pixel \( p \), respectively, and \( n \) is the total number of pixels.

To verify the scale-invariance property, consider scaling the predicted depths by a positive constant \( \alpha \), replacing \( \hat{d}_p \) with \( \alpha \hat{d}_p \). The loss becomes:
\begin{equation}
    L(\alpha \hat{d}, d) = \frac{1}{n} \sum_{p} \left( \ln (\alpha \hat{d}_p) - \ln d_p \right)^2 - \frac{1}{n^2} \left( \sum_{p} \left( \ln (\alpha \hat{d}_p) - \ln d_p \right) \right)^2.
\end{equation}

Using the identity \( \ln (\alpha \hat{d}_p) = \ln \alpha + \ln \hat{d}_p \), we rewrite the expression:
\begin{equation}
    = \frac{1}{n} \sum_{p} \left( \ln \alpha + \ln \frac{\hat{d}_p}{d_p} \right)^2 - \frac{1}{n^2} \left( \sum_{p} \left( \ln \alpha + \ln \frac{\hat{d}_p}{d_p} \right) \right)^2.
\end{equation}

Let \( \beta = \ln \alpha \), a constant. Expanding both terms:
\begin{align}
    L(\alpha \hat{d}, d) &= \frac{1}{n} \sum_{p} \left( \beta^2 + 2\beta \ln \frac{\hat{d}_p}{d_p} + \left( \ln \frac{\hat{d}_p}{d_p} \right)^2 \right) \\
    &\quad - \frac{1}{n^2} \left( \beta n + \sum_{p} \ln \frac{\hat{d}_p}{d_p} \right)^2.
\end{align}

Simplifying, we find that all terms involving \( \beta \) cancel out:
\begin{equation}
    L(\alpha \hat{d}, d) = \frac{1}{n} \sum_{p} \left( \ln \frac{\hat{d}_p}{d_p} \right)^2 - \frac{1}{n^2} \left( \sum_{p} \ln \frac{\hat{d}_p}{d_p} \right)^2.
\end{equation}

Thus, the loss function remains unchanged under uniform scaling of the predicted depth values. This proves that the Scale-Invariant Logarithmic Loss is indeed invariant to global scale, making it especially suitable for tasks where relative depth relationships are more important than absolute depth values.
